# Supplementary material for: Nonequilibrium Kondo effect in a graphene-coupled quantum dot in the presence of a magnetic field
Source: arXiv:1902.09924 ancillary file (2020-01-29)
Supplement: Supplementary file 1 [file Supporting_Information_File_1.pdf]

# Supporting Information
for
# Nonequilibrium Kondo effect in a graphene-coupled quantum dot in the presence of a magnetic field

Levente Máthé[1, 2, *] and Ioan Grosu[2]

[1] *Department of Molecular and Biomolecular Physics, National Institute for Research and Development of Isotopic and Molecular Technologies, 67-103 Donath, 400293 Cluj-Napoca, Romania*

[2] *Faculty of Physics, Babeș-Bolyai University, 1 Kogălniceanu, 400084 Cluj-Napoca, Romania*

* Corresponding author: levente.mathe@itim-cj.ro

### Appendix A: Green's function of the dot

The retarded Green's function is defined as $\langle\langle A(t)|B(0)\rangle\rangle^r_t = -i\theta(t)\langle\{A(t), B(0)\}\rangle$, where $A$ and $B$ are fermionic operators and $\theta(t)$ is the Heaviside function [1–3]. Its Fourier transform reads $\langle\langle A|B\rangle\rangle^r_\omega$. The equation of motion of the retarded Green's function in energy space is $\omega^+\langle\langle A|B\rangle\rangle^r_\omega + \langle\langle [H, A]|B\rangle\rangle^r_\omega = \langle\{A, B\}\rangle$ where $\omega^+ = \omega + i\delta$, with $\delta$ being a positive infinitesimal [1, 3]. We can define the dot retarded Green's function as $G^r_{d\sigma}(\omega) = \langle\langle d_\sigma|d^\dagger_\sigma\rangle\rangle^r_\omega$ when replacing $A(B)$ by $d_\sigma(d^\dagger_\sigma)$ in the above notations. The equation of motion for $G^r_{d\sigma}(\omega)$ is:

$$(\omega^+ - \varepsilon_{d\sigma})G^r_{d\sigma}(\omega) = 1 + U\langle\langle d_\sigma n_{\bar\sigma}|d^\dagger_\sigma\rangle\rangle^r_\omega + \sum_{\alpha,s}\int_{-k_c}^{+k_c} dk V(k)\langle\langle c_{\alpha sk\sigma}|d^\dagger_\sigma\rangle\rangle^r_\omega. \tag{S1}$$

The equation for the term $\langle\langle c_{\alpha sk\sigma}|d^\dagger_\sigma\rangle\rangle^r_\omega$ reads:

$$\langle\langle c_{\alpha sk\sigma}|d^\dagger_\sigma\rangle\rangle^r_\omega = \frac{V(k)}{\omega^+ - \varepsilon_k}\langle\langle d_\sigma|d^\dagger_\sigma\rangle\rangle^r_\omega. \tag{S2}$$

We define the $\Sigma^r_0(\omega)$ self-energy as:

$$\Sigma^r_0(\omega) = \sum_{\alpha,s}\int_{-k_c}^{+k_c} dk\frac{V(k)^2}{\omega^+ - \varepsilon_k} = -2\eta\Big(\omega\ln\Big|\frac{D^2-\omega^2}{\omega^2}\Big| + i\pi|\omega|\theta(D-|\omega|)\Big), \tag{S3}$$

where we used the Eq. (S31) and introduced a dimensionless parameter as $\eta = 2(\tilde V/\hbar v_F)^2$. By substituting Eq. (S2) into Eq. (S1) with Eq. (S3) we have:

$$(\omega^+ - \varepsilon_{d\sigma} - \Sigma^r_0(\omega))G^r_{d\sigma}(\omega) = 1 + U\langle\langle d_\sigma n_{\bar\sigma}|d^\dagger_\sigma\rangle\rangle^r_\omega. \tag{S4}$$

The equation of motion for $\langle\langle d_\sigma n_{\bar\sigma}|d^\dagger_\sigma\rangle\rangle^r_\omega$ is:

$$\begin{aligned}(\omega^+ - \varepsilon_{d\sigma} - U)\langle\langle d_\sigma n_{\bar\sigma}|d^\dagger_\sigma\rangle\rangle^r_\omega &= \langle n_{\bar\sigma}\rangle\\ &+ \sum_{\alpha,s}\int_{-k_c}^{+k_c} dkV(k)\Big[\langle\langle c_{\alpha sk\sigma}n_{\bar\sigma}|d^\dagger_\sigma\rangle\rangle^r_\omega + \langle\langle d^\dagger_{\bar\sigma}c_{\alpha sk\bar\sigma}d_\sigma|d^\dagger_\sigma\rangle\rangle^r_\omega - \langle\langle c^\dagger_{\alpha sk\bar\sigma}d_{\bar\sigma}d_\sigma|d^\dagger_\sigma\rangle\rangle^r_\omega\Big].\end{aligned} \tag{S5}$$

To determine the Green's function of the quantum dot, we need to calculate the new higher-order correlation functions that appear on the right-hand side of Eq. (S5). The equations of motion for these terms are expressed as:

$$\begin{aligned}\Omega^{(0)}_k(\omega)\langle\langle c_{\alpha sk\sigma}n_{\bar\sigma}|d^\dagger_\sigma\rangle\rangle^r_\omega &= V(k)\langle\langle d_\sigma n_{\bar\sigma}|d^\dagger_\sigma\rangle\rangle^r_\omega\\ &- \sum_{\alpha',s'}\int_{-k_c}^{+k_c} dk'V(k')\Big[\langle\langle c_{\alpha sk\sigma}c^\dagger_{\alpha's'k'\bar\sigma}d_{\bar\sigma}|d^\dagger_\sigma\rangle\rangle^r_\omega + \langle\langle c_{\alpha sk\sigma}c_{\alpha's'k'\bar\sigma}d^\dagger_{\bar\sigma}|d^\dagger_\sigma\rangle\rangle^r_\omega\Big],\end{aligned} \tag{S6}$$

$$\begin{aligned}\Omega^{(1)}_{k\sigma}(\omega)\langle\langle d^\dagger_{\bar\sigma}c_{\alpha sk\bar\sigma}d_\sigma|d^\dagger_\sigma\rangle\rangle^r_\omega &= \langle d^\dagger_{\bar\sigma}c_{\alpha sk\bar\sigma}\rangle + V(k)\langle\langle d_\sigma n_{\bar\sigma}|d^\dagger_\sigma\rangle\rangle^r_\omega\\ &+ \sum_{\alpha',s'}\int_{-k_c}^{+k_c} dk'V(k')\Big[\langle\langle d^\dagger_{\bar\sigma}c_{\alpha sk\bar\sigma}c_{\alpha's'k'\sigma}|d^\dagger_\sigma\rangle\rangle^r_\omega - \langle\langle c^\dagger_{\alpha's'k'\bar\sigma}c_{\alpha sk\bar\sigma}d_\sigma|d^\dagger_\sigma\rangle\rangle^r_\omega\Big],\end{aligned} \tag{S7}$$

$$\begin{aligned}\Omega^{(2)}_{k\sigma}(\omega)\langle\langle c^\dagger_{\alpha sk\bar\sigma}d_{\bar\sigma}d_\sigma|d^\dagger_\sigma\rangle\rangle^r_\omega &= \langle c^\dagger_{\alpha sk\bar\sigma}d_{\bar\sigma}\rangle - V(k)\langle\langle d_\sigma n_{\bar\sigma}|d^\dagger_\sigma\rangle\rangle^r_\omega\\ &+ \sum_{\alpha',s'}\int_{-k_c}^{+k_c} dk'V(k')\Big[\langle\langle c^\dagger_{\alpha sk\bar\sigma}c_{\alpha's'k'\bar\sigma}d_\sigma|d^\dagger_\sigma\rangle\rangle^r_\omega - \langle\langle c^\dagger_{\alpha sk\bar\sigma}c_{\alpha's'k'\sigma}d_{\bar\sigma}|d^\dagger_\sigma\rangle\rangle^r_\omega\Big],\end{aligned} \tag{S8}$$

where the following notations are used: $\Omega^{(0)}_k(\omega) \equiv \omega^+ - \varepsilon_k$, $\Omega^{(1)}_{k\sigma}(\omega) \equiv \omega^+ - \varepsilon_k + (\varepsilon_{d\bar\sigma} - \varepsilon_{d\sigma})$ and $\Omega^{(2)}_{k\sigma}(\omega) \equiv \omega^+ + \varepsilon_k - (\varepsilon_{d\bar\sigma} + \varepsilon_{d\sigma}) - U$. To obtain an analytical formula for the Green's function of the quantum dot, we have to truncate the higher-order correlation functions that appear in Eqs. (S6)-(S8) by using an approximation method. In order to do

this, we apply the broadly used Lacroix decoupling scheme [2] that leads to close the infinite number of higher-order correlation functions. By performing the approximations and substituting the resulting equations into the Eq. (S5) for the Green's function of the quantum dot, we obtain:

$$G^r_{d\sigma}(\omega) = \frac{\Pi^{(1)}_\sigma(\omega) + U\big[\langle n_{\bar\sigma}\rangle + \Pi^{(2)}_\sigma(\omega)\big]}{\Pi^{(1)}_\sigma(\omega)\big[\omega - \varepsilon_{d\sigma} - \Sigma^r_0(\omega)\big] - U\Pi^{(3)}_\sigma(\omega)}, \tag{S9}$$

where we introduced the notations:

$$\Pi^{(1)}_\sigma(\omega) = \omega - \varepsilon_{d\sigma} - U - \Sigma^r_0(\omega) - \sum_{\alpha,s}\int_{-k_c}^{+k_c} dk V(k)^2\left[\frac{1}{\Omega^{(1)}_{k\sigma}} + \frac{1}{\Omega^{(2)}_{k\sigma}}\right], \tag{S10}$$

$$\Pi^{(2)}_\sigma(\omega) = \sum_{\alpha,s}\int_{-k_c}^{+k_c} dk V(k)\left[\frac{\langle d^\dagger_{\bar\sigma} c_{\alpha sk\bar\sigma}\rangle}{\Omega^{(1)}_{k\sigma}} - \frac{\langle c^\dagger_{\alpha sk\bar\sigma} d_{\bar\sigma}\rangle}{\Omega^{(2)}_{k\sigma}}\right], \tag{S11}$$

$$\Pi^{(3)}_\sigma(\omega) = \Sigma^r_0(\omega)\Pi^{(2)}_\sigma(\omega) - \sum_{\substack{\alpha,s\\ \alpha',s'}}\iint_{-k_c}^{+k_c} dk dk' V(k)V(k')\left[\frac{\langle c^\dagger_{\alpha' s' k'\bar\sigma} c_{\alpha sk\bar\sigma}\rangle}{\Omega^{(1)}_{k\sigma}} + \frac{\langle c^\dagger_{\alpha sk\bar\sigma} c_{\alpha' s' k'\bar\sigma}\rangle}{\Omega^{(2)}_{k\sigma}}\right]. \tag{S12}$$

The average values of the mixing operators in the above relations are treated non-self-consistently, following the Meir approximation [4], i.e. $\langle d^\dagger_{\bar\sigma} c_{\alpha sk\bar\sigma}\rangle = \langle c^\dagger_{\alpha sk\bar\sigma} d_{\bar\sigma}\rangle \approx 0$ and $\langle c^\dagger_{\alpha' s' k'\bar\sigma} c_{\alpha sk\bar\sigma}\rangle = \langle c^\dagger_{\alpha sk\bar\sigma} c_{\alpha' s' k'\bar\sigma}\rangle \approx f_\alpha(\varepsilon_k)\delta_{\alpha\alpha'}\delta_{ss'}\delta(k-k')$. In this case $\Pi^{(2)}_\sigma(\omega) \approx 0$, the retarded Green's function for the quantum dot reduces:

$$\begin{aligned} G^r_{d\sigma}(\omega) = {}& \frac{1 - \langle n_{\bar\sigma}\rangle}{\omega - \varepsilon_{d\sigma} - \Sigma^r_0(\omega) + U\frac{\Sigma_{3\sigma}(\omega)+\Sigma_{4\sigma}(\omega)}{\omega-\varepsilon_{d\sigma}-U-\Sigma^r_0(\omega)-\Sigma_{1\sigma}(\omega)-\Sigma_{2\sigma}(\omega)}} \\ & + \frac{\langle n_{\bar\sigma}\rangle}{\omega - \varepsilon_{d\sigma} - \Sigma^r_0(\omega) - U - U\frac{\Sigma_{1\sigma}(\omega)+\Sigma_{2\sigma}(\omega)-\Sigma_{3\sigma}(\omega)-\Sigma_{4\sigma}(\omega)}{\omega-\varepsilon_{d\sigma}-\Sigma^r_0(\omega)-\Sigma_{1\sigma}(\omega)-\Sigma_{2\sigma}(\omega)}}, \end{aligned} \tag{S13}$$

where we defined the following self-energies by the relations:

$$\Sigma_{i\sigma}(\omega) = \sum_{\alpha,s}\int_{-k_c}^{+k_c} dk\frac{V(k)^2}{\Omega^{(i)}_{k\sigma}(\omega)} = -2\eta\left[\omega_{i\sigma}\ln\left|\frac{D^2-\omega^2_{i\sigma}}{\omega^2_{i\sigma}}\right| + i\pi|\omega_{i\sigma}|\theta(D-|\omega_{i\sigma}|)\right], \quad i = 1,2, \tag{S14}$$

with shorthand notations: $\omega_{1\sigma} = \omega - \sigma\Delta\varepsilon_d$ and $\omega_{2\sigma} = \omega - 2\varepsilon_d - U$. Therefore, we have $\Sigma_{3\sigma}(\omega) = \sum_{\alpha,s}\int_{-k_c}^{+k_c} dk V(k)^2\Omega^{(1)}_{k\sigma}(\omega)^{-1} f_\alpha(\varepsilon_k) = \sum_\alpha \Sigma^{\alpha(\gamma)}_{3\sigma}(\omega)$ and $\Sigma_{4\sigma}(\omega) = \sum_{\alpha,s}\int_{-k_c}^{+k_c} dk V(k)^2\Omega^{(2)}_{k\sigma}(\omega)^{-1} f_\alpha(\varepsilon_k)$ $= \sum_\alpha \Sigma^{\alpha(\gamma)}_{4\sigma}(\omega)$ with solutions:

$$\Sigma^{\alpha(-)}_{3\sigma}(\omega) = \eta\left[D + \omega_{1\sigma}\ln\left|\frac{\mu_\alpha - \omega_{1\sigma} - 2T}{D+\omega_{1\sigma}}\right| - R^\alpha_{3\sigma}(\omega) - iJ^\alpha_{3\sigma}(\omega)\right], \tag{S15}$$

$$\Sigma^{\alpha(0)}_{3\sigma}(\omega) = \eta\left\{D - T + \omega_{1\sigma}\ln\left|\frac{\omega_{1\sigma}+2T}{D+\omega_{1\sigma}}\right| - \frac{\omega_{1\sigma}}{2}\left(1 - \frac{\omega_{1\sigma}}{2T}\right)\ln\left|\frac{(\omega_{1\sigma}+2T)(\omega_{1\sigma}-2T)}{\omega^2_{1\sigma}}\right| - iJ^\alpha_{3\sigma}(\omega)\right\}, \tag{S16}$$

$$\Sigma^{\alpha(+)}_{3\sigma}(\omega) = \eta\left[D - \omega_{1\sigma}\ln\left|\frac{(D+\omega_{1\sigma})(\mu_\alpha - \omega_{1\sigma} - 2T)}{\omega^2_{1\sigma}}\right| + R^\alpha_{3\sigma}(\omega) - iJ^\alpha_{3\sigma}(\omega)\right], \tag{S17}$$

where we introduced the following relations:

$$R^\alpha_{3\sigma}(\omega) = \omega_{1\sigma} - \mu_\alpha + \frac{\omega_{1\sigma}}{2}\left(1 + \frac{\mu_\alpha - \omega_{1\sigma}}{2T}\right)\ln\left|\frac{\mu_\alpha - \omega_{1\sigma} - 2T}{\mu_\alpha - \omega_{1\sigma} + 2T}\right|, \tag{S18}$$

$$J^\alpha_{3\sigma}(\omega) = \frac{\pi}{2}|\omega_{1\sigma}|\left[1 + \tanh\left(\frac{\mu_\alpha - \omega_{1\sigma}}{2T}\right)\right]\theta(D+\omega_{1\sigma}) \tag{S19}$$

and:

$$\Sigma^{\alpha(-)}_{4\sigma}(\omega) = -\eta\Big[D + \omega_{2\sigma}\ln\Big|\frac{D-\omega_{2\sigma}}{\mu_\alpha+\omega_{2\sigma}-2T}\Big| + R^{\alpha}_{4\sigma}(\omega) + iJ^{\alpha}_{4\sigma}(\omega)\Big], \tag{S20}$$

$$\Sigma^{\alpha(0)}_{4\sigma}(\omega) = -\eta\Big\{D - T + \omega_{2\sigma}\ln\Big|\frac{D-\omega_{2\sigma}}{\omega_{2\sigma}-2T}\Big| + \frac{\omega_{2\sigma}}{2}\Big(1+\frac{\omega_{2\sigma}}{2T}\Big)\ln\Big|\frac{(\omega_{2\sigma}-2T)(\omega_{2\sigma}+2T)}{\omega_{2\sigma}^2}\Big| + iJ^{\alpha}_{4\sigma}(\omega)\Big\}, \tag{S21}$$

$$\Sigma^{\alpha(+)}_{4\sigma}(\omega) = -\eta\Big[D + \omega_{2\sigma}\ln\Big|\frac{(D-\omega_{2\sigma})(\mu_\alpha+\omega_{2\sigma}-2T)}{\omega_{2\sigma}^2}\Big| - R^{\alpha}_{4\sigma}(\omega) + iJ^{\alpha}_{4\sigma}(\omega)\Big], \tag{S22}$$

where we have:

$$R^{\alpha}_{4\sigma}(\omega) = \omega_{2\sigma} + \mu_\alpha + \frac{\omega_{2\sigma}}{2}\Big(1+\frac{\mu_\alpha+\omega_{2\sigma}}{2T}\Big)\ln\Big|\frac{\mu_\alpha+\omega_{2\sigma}-2T}{\mu_\alpha+\omega_{2\sigma}+2T}\Big|, \tag{S23}$$

$$J^{\alpha}_{4\sigma}(\omega) = \frac{\pi}{2}|\omega_{2\sigma}|\Big[1+\tanh\Big(\frac{\mu_\alpha+\omega_{2\sigma}}{2T}\Big)\Big]\theta(D-\omega_{2\sigma}), \tag{S24}$$

where $\gamma = -, 0$ and $+$ correspond to the cases: $-D < \mu_\alpha \lesssim 0$, $\mu_\alpha = 0$ and $0 \lesssim \mu_\alpha < D$.

### Appendix B: Derivation of the self-energies at finite temperature

In this section, we show a simple method to deduce self-energies $\Sigma_{3\sigma}(\omega)$ and $\Sigma_{4\sigma}(\omega)$ for finite temperatures. We introduce the self-energies by:

$$\Sigma_{3\sigma}(\omega) = \sum_{\alpha,s}\int_{-k_c}^{+k_c} dk\frac{V(k)^2}{\Omega^{(1)}_{k\sigma}(\omega)}f(\varepsilon_k-\mu_\alpha) = \sum_{\alpha}\Sigma^{\alpha(\gamma)}_{3\sigma}(\omega) \tag{S25}$$

and:

$$\Sigma_{4\sigma}(\omega) = \sum_{\alpha,s}\int_{-k_c}^{+k_c} dk\frac{V(k)^2}{\Omega^{(2)}_{k\sigma}(\omega)}f(\varepsilon_k-\mu_\alpha) = \sum_{\alpha}\Sigma^{\alpha(\gamma)}_{4\sigma}(\omega), \tag{S26}$$

with:

$$\Sigma^{\alpha(\gamma)}_{3\sigma}(\omega) = \eta\int_{-D}^{+D} d\varepsilon\frac{|\varepsilon|f(\varepsilon-\mu_\alpha)}{-\varepsilon+\omega_{1\sigma}+i\delta} = \eta I^{\alpha(\gamma)}_{3\sigma}(\omega) \tag{S27}$$

and:

$$\Sigma^{\alpha(\gamma)}_{4\sigma}(\omega) = \eta\int_{-D}^{+D} d\varepsilon\frac{|\varepsilon|f(\varepsilon-\mu_\alpha)}{\varepsilon+\omega_{2\sigma}+i\delta} = \eta I^{\alpha(\gamma)}_{4\sigma}(\omega), \tag{S28}$$

where we introduced the notation $\varepsilon = \hbar v_F k$. Note that $\Sigma^{\alpha(\gamma)}_{3\sigma}(\omega)$ and $\Sigma^{\alpha(\gamma)}_{4\sigma}(\omega)$ explicitly depend on $\omega$ through $\omega_{1\sigma}$ and $\omega_{2\sigma}$, respectively. Furthermore, by changing the variable $\beta(\varepsilon-\mu_\alpha) = x$ where $\beta = 1/T$, then the Fermi function $f(\varepsilon-\mu_\alpha)$ can be expressed as:

$$f(x) = \frac{1}{2}\Big[1-\tanh\Big(\frac{x}{2}\Big)\Big], \tag{S29}$$

where $\tanh(x/2)$ has the properties [5]:

$$\tanh\Big(\frac{x}{2}\Big) \approx \begin{cases} -1 & \text{if } x < -2 \\ \frac{x}{2} & \text{if } -2 < x < 2 \\ +1 & \text{if } x > 2. \end{cases} \tag{S30}$$

The following calculations will be based on the properties of function $\tanh(x/2)$ outlined in Eq. (S30). We also use the Dirac identity [6]:

$$\frac{1}{x \pm i\eta} = \mathcal{P}\frac{1}{x} \mp i\pi\delta(x), \tag{S31}$$

where $\eta$ is a positive infinitesimal, $\mathcal{P}$ is the Cauchy principal value and $\delta(x)$ being the Dirac delta function. We implicity applied this relation to deduce $\Sigma_0^r(\omega)$ and $\Sigma_{i\sigma}(\omega)$ in Eqs. (S3) and (S14). From Eq. (S27) we write for $I_{3\sigma}^{\alpha(\gamma)}(\omega) = I_{3\sigma}^{\alpha(\gamma)1}(\omega) - I_{3\sigma}^{\alpha(\gamma)2}(\omega)$ with:

$$I_{3\sigma}^{\alpha(\gamma)1}(\omega) = \int_{-D}^{0} d\varepsilon \frac{\varepsilon \cdot f(\varepsilon - \mu_\alpha)}{\varepsilon - \omega_{1\sigma} - i\delta}, \tag{S32}$$

$$I_{3\sigma}^{\alpha(\gamma)2}(\omega) = \int_{0}^{D} d\varepsilon \frac{\varepsilon \cdot f(\varepsilon - \mu_\alpha)}{\varepsilon - \omega_{1\sigma} - i\delta}. \tag{S33}$$

Firstly, we assume that $0 \lesssim \mu_\alpha < D$ and $0 \lesssim \omega_{1\sigma} < D'$ where $D' > D$ is arbitrarily introduced. Using Eqs. (S29)-(S31) then $I_{3\sigma}^{\alpha(+)1}(\omega)$ and $I_{3\sigma}^{\alpha(+)2}(\omega)$ can be calculated as:

$$I_{3\sigma}^{\alpha(+)1}(\omega) \approx \frac{1}{2\beta}\int_{-\beta(D+\mu_\alpha)}^{-\beta\mu_\alpha} \frac{dx(x+\beta\mu_\alpha)}{x+\beta(\mu_\alpha - \omega_{1\sigma})}\Big[1 - \tanh\Big(\frac{x}{2}\Big)\Big] \approx D + \omega_{1\sigma}\ln\left|\frac{\omega_{1\sigma}}{D+\omega_{1\sigma}}\right|, \tag{S34}$$

where the imaginary part in the integral has been neglected due to the limits of integration, and:

$$\begin{aligned} I_{3\sigma}^{\alpha(+)2}(\omega) &= \frac{1}{2\beta}\int_{-\beta\mu_\alpha}^{\beta(D-\mu_\alpha)} \frac{dx(x+\beta\mu_\alpha)}{x+\beta(\mu_\alpha - \omega_{1\sigma}) - i\eta}\Big[1 - \tanh\Big(\frac{x}{2}\Big)\Big] \\ &\approx -\omega_{1\sigma}\ln\left|\frac{\omega_{1\sigma}}{\mu_\alpha - \omega_{1\sigma} - 2T}\right| - \frac{\omega_{1\sigma}}{2}\Big(1 + \frac{\mu_\alpha - \omega_{1\sigma}}{2T}\Big)\ln\left|\frac{\mu_\alpha - \omega_{1\sigma} - 2T}{\mu_\alpha - \omega_{1\sigma} + 2T}\right| \\ &+ \mu_\alpha - \omega_{1\sigma} + i\frac{\pi}{2}\omega_{1\sigma}\Big[1 + \tanh\Big(\frac{\mu_\alpha - \omega_{1\sigma}}{2T}\Big)\Big], \end{aligned} \tag{S35}$$

where $\eta = \delta\beta \to 0^+$. We consider the case: $0 \lesssim \mu_\alpha < D$ and $-D' < \omega_{1\sigma} \lesssim 0$. Introducing $\omega_{1\sigma}^+ = -\omega_{1\sigma}$ in the same way we find:

$$\begin{aligned} I_{3\sigma}^{\alpha(+)1}(\omega) &= \frac{1}{2\beta}\int_{-\beta(D+\mu_\alpha)}^{-\beta\mu_\alpha} \frac{dx(x+\beta\mu_\alpha)}{x+\beta(\mu_\alpha + \omega_{1\sigma}^+) - i\eta}\Big[1 - \tanh\Big(\frac{x}{2}\Big)\Big] \\ &\approx D - \omega_{1\sigma}^+\ln\left|\frac{\omega_{1\sigma}^+}{D - \omega_{1\sigma}^+}\right| - i\frac{\pi}{2}\omega_{1\sigma}^+\Big[1 + \tanh\Big(\frac{\mu_\alpha + \omega_{1\sigma}^+}{2T}\Big)\Big]\theta(D - \omega_{1\sigma}^+). \end{aligned} \tag{S36}$$

Furthermore, we have:

$$\begin{aligned} I_{3\sigma}^{\alpha(+)2}(\omega) &\approx \frac{1}{2\beta}\int_{-\beta\mu_\alpha}^{\beta(D-\mu_\alpha)} \frac{dx(x+\beta\mu_\alpha)}{x+\beta(\mu_\alpha + \omega_{1\sigma}^+)}\Big[1 - \tanh\Big(\frac{x}{2}\Big)\Big] \approx \mu_\alpha + \omega_{1\sigma}^+ \\ &+ \omega_{1\sigma}^+\ln\left|\frac{\omega_{1\sigma}^+}{\mu_\alpha + \omega_{1\sigma}^+ - 2T}\right| - \frac{\omega_{1\sigma}^+}{2}\Big(1 + \frac{\mu_\alpha + \omega_{1\sigma}^+}{2T}\Big)\ln\left|\frac{\mu_\alpha + \omega_{1\sigma}^+ + 2T}{\mu_\alpha + \omega_{1\sigma}^+ - 2T}\right|. \end{aligned} \tag{S37}$$

Combining Eqs. (S34)-(S37) we simply obtain $I_{3\sigma}^{\alpha(+)}$ defined for the full range of the energy, $-D' < \omega_{1\sigma} < D'$:

$$\begin{aligned} I_{3\sigma}^{\alpha(+)}(\omega) &\approx D - \mu_\alpha + \omega_{1\sigma} - \omega_{1\sigma}\ln\left|\frac{(D+\omega_{1\sigma})(\mu_\alpha - \omega_{1\sigma} - 2T)}{\omega_{1\sigma}^2}\right| + \frac{\omega_{1\sigma}}{2}\Big(1 + \frac{\mu_\alpha - \omega_{1\sigma}}{2T}\Big)\ln\left|\frac{\mu_\alpha - \omega_{1\sigma} - 2T}{\mu_\alpha - \omega_{1\sigma} + 2T}\right| \\ &- i\frac{\pi}{2}|\omega_{1\sigma}|\Big[1 + \tanh\Big(\frac{\mu_\alpha - \omega_{1\sigma}}{2T}\Big)\Big]\theta(D + \omega_{1\sigma}). \end{aligned} \tag{S38}$$

Assuming that $-D < \mu_\alpha \lesssim 0$ and $0 \lesssim \omega_{1\sigma} < D'$ and introducing $\mu_\alpha^+ = -\mu_\alpha$, thus, one finds:

$$\begin{aligned} I_{3\sigma}^{\alpha(-)1}(\omega) &\approx \frac{1}{2\beta}\int_{-\beta(D-\mu_\alpha^+)}^{\beta\mu_\alpha^+} \frac{dx(x-\beta\mu_\alpha^+)}{x-\beta(\mu_\alpha^+ + \omega_{1\sigma})}\Big[1 - \tanh\Big(\frac{x}{2}\Big)\Big] \approx D - \mu_\alpha^+ - \omega_{1\sigma} \\ &+ \omega_{1\sigma}\ln\left|\frac{\mu_\alpha^+ + \omega_{1\sigma} + 2T}{D + \omega_{1\sigma}}\right| + \frac{\omega_{1\sigma}}{2}\Big(1 - \frac{\mu_\alpha^+ + \omega_{1\sigma}}{2T}\Big)\ln\left|\frac{\mu_\alpha^+ + \omega_{1\sigma} - 2T}{\mu_\alpha^+ + \omega_{1\sigma} + 2T}\right|, \end{aligned} \tag{S39}$$

$$I_{3\sigma}^{\alpha(-)2}(\omega)=\frac{1}{2\beta}\int_{\beta\mu_\alpha^+}^{\beta(D+\mu_\alpha^+)}\frac{dx(x-\beta\mu_\alpha^+)}{x-\beta(\mu_\alpha^++\omega_{1\sigma})-i\eta}\Big[1-\tanh\Big(\frac{x}{2}\Big)\Big]\approx i\frac{\pi}{2}\omega_{1\sigma}\Big[1-\tanh\Big(\frac{\mu_\alpha^++\omega_{1\sigma}}{2T}\Big)\Big]. \tag{S40}$$

In the case of $-D<\mu_\alpha\lesssim 0$, $-D'<\omega_{1\sigma}\lesssim 0$ and introducing $\mu_\alpha^+=-\mu_\alpha$ and $\omega_{1\sigma}^+=-\omega_{1\sigma}$ we have:

$$\begin{aligned}I_{3\sigma}^{\alpha(-)1}(\omega)&=\frac{1}{2\beta}\int_{-\beta(D-\mu_\alpha^+)}^{\beta\mu_\alpha^+}\frac{dx(x-\beta\mu_\alpha^+)}{x-\beta(\mu_\alpha^+-\omega_{1\sigma}^+)-i\eta}\Big[1-\tanh\Big(\frac{x}{2}\Big)\Big]\approx D-\mu_\alpha^++\omega_{1\sigma}^+-\omega_{1\sigma}^+\ln\Big|\frac{\mu_\alpha^+-\omega_{1\sigma}^++2T}{D-\omega_{1\sigma}^+}\Big|\\&-\frac{\omega_{1\sigma}^+}{2}\Big(1-\frac{\mu_\alpha^+-\omega_{1\sigma}^+}{2T}\Big)\ln\Big|\frac{\mu_\alpha^+-\omega_{1\sigma}^+-2T}{\mu_\alpha^+-\omega_{1\sigma}^++2T}\Big|-i\frac{\pi}{2}\omega_{1\sigma}^+\Big[1-\tanh\Big(\frac{\mu_\alpha^+-\omega_{1\sigma}^+}{2T}\Big)\Big]\theta(D-\omega_{1\sigma}^+),\end{aligned} \tag{S41}$$

$$I_{3\sigma}^{\alpha(-)2}(\omega)\approx\frac{1}{2\beta}\int_{\beta\mu_\alpha^+}^{\beta(D+\mu_\alpha^+)}\frac{dx(x-\beta\mu_\alpha^+)}{x-\beta(\mu_\alpha^+-\omega_{1\sigma}^+)}\Big[1-\tan\Big(\frac{x}{2}\Big)\Big]\approx 0. \tag{S42}$$

Comparing Eqs. (S39)-(S40) with Eqs. (S41)-(S42) one finds the $I_{3\sigma}^{\alpha(-)}$ for the entire energy domain, $-D'<\omega_{1\sigma}<D'$:

$$\begin{aligned}I_{3\sigma}^{\alpha(-)}(\omega)&\approx D+\mu_\alpha-\omega_{1\sigma}+\omega_{1\sigma}\ln\Big|\frac{\mu_\alpha-\omega_{1\sigma}-2T}{D+\omega_{1\sigma}}\Big|+\frac{\omega_{1\sigma}}{2}\Big(1+\frac{\mu_\alpha-\omega_{1\sigma}}{2T}\Big)\ln\Big|\frac{\mu_\alpha-\omega_{1\sigma}+2T}{\mu_\alpha-\omega_{1\sigma}-2T}\Big|\\&-i\frac{\pi}{2}|\omega_{1\sigma}|\Big[1+\tanh\Big(\frac{\mu_\alpha-\omega_{1\sigma}}{2T}\Big)\Big]\theta(D+\omega_{1\sigma}).\end{aligned} \tag{S43}$$

Now, we consider the case $\mu_\alpha=0$ and $0\lesssim\omega_{1\sigma}<D'$ and find:

$$\begin{aligned}I_{3\sigma}^{\alpha(0)1}(\omega)&\approx\frac{1}{2\beta}\int_{-\beta D}^{0}\frac{xdx}{x-\beta\omega_{1\sigma}}\Big[1-\tanh\Big(\frac{x}{2}\Big)\Big]\\&\approx D+\omega_{1\sigma}\ln\Big|\frac{\omega_{1\sigma}+2T}{D+\omega_{1\sigma}}\Big|+\frac{\omega_{1\sigma}}{2}\Big(1-\frac{\omega_{1\sigma}}{2T}\Big)\ln\Big|\frac{\omega_{1\sigma}}{\omega_{1\sigma}+2T}\Big|-\frac{T}{2}-\frac{\omega_{1\sigma}}{2},\end{aligned} \tag{S44}$$

$$\begin{aligned}I_{3\sigma}^{\alpha(0)2}(\omega)&=\frac{1}{2\beta}\int_{0}^{\beta D}\frac{xdx}{x-\beta\omega_{1\sigma}-i\eta}\Big[1-\tanh\Big(\frac{x}{2}\Big)\Big]\approx\frac{T}{2}-\frac{\omega_{1\sigma}}{2}\\&+\frac{\omega_{1\sigma}}{2}\Big(1-\frac{\omega_{1\sigma}}{2T}\Big)\ln\Big|\frac{\omega_{1\sigma}-2T}{\omega_{1\sigma}}\Big|+i\frac{\pi}{2}\omega_{1\sigma}\Big[1-\tanh\Big(\frac{\omega_{1\sigma}}{2T}\Big)\Big].\end{aligned} \tag{S45}$$

For $\mu_\alpha=0$ and $-D'<\omega_{1\sigma}\lesssim 0$ with $\omega_{1\sigma}^+=-\omega_{1\sigma}$ we have:

$$\begin{aligned}I_{3\sigma}^{\alpha(0)1}(\omega)&=\frac{1}{2\beta}\int_{-\beta D}^{0}\frac{xdx}{x+\beta\omega_{1\sigma}^+-i\eta}\Big[1-\tanh\Big(\frac{x}{2}\Big)\Big]\approx D-\frac{T}{2}+\frac{\omega_{1\sigma}^+}{2}+\omega_{1\sigma}^+\ln\Big|\frac{\omega_{1\sigma}^+-D}{\omega_{1\sigma}^+-2T}\Big|\\&-\frac{\omega_{1\sigma}^+}{2}\Big(1+\frac{\omega_{1\sigma}^+}{2T}\Big)\ln\Big|\frac{\omega_{1\sigma}^+}{\omega_{1\sigma}^+-2T}\Big|-i\frac{\pi}{2}\omega_{1\sigma}^+\Big[1+\tanh\Big(\frac{\omega_{1\sigma}^+}{2T}\Big)\Big]\theta(D-\omega_{1\sigma}^+),\end{aligned} \tag{S46}$$

$$I_{3\sigma}^{\alpha(0)2}(\omega)\approx\frac{1}{2\beta}\int_{0}^{\beta D}\frac{xdx}{x+\beta\omega_{1\sigma}^+}\Big[1-\tanh\Big(\frac{x}{2}\Big)\Big]\approx\frac{T}{2}+\frac{\omega_{1\sigma}^+}{2}-\frac{\omega_{1\sigma}^+}{2}\Big(1+\frac{\omega_{1\sigma}^+}{2T}\Big)\ln\Big|\frac{\omega_{1\sigma}^++2T}{\omega_{1\sigma}^+}\Big|. \tag{S47}$$

Using Eqs. (S44)-(S47) for the full energy domain $I_{3\sigma}^{\alpha(0)}$ can be expressed as:

$$\begin{aligned}I_{3\sigma}^{\alpha(0)}(\omega)&\approx D-T+\omega_{1\sigma}\ln\Big|\frac{\omega_{1\sigma}+2T}{D+\omega_{1\sigma}}\Big|-\frac{\omega_{1\sigma}}{2}\Big(1-\frac{\omega_{1\sigma}}{2T}\Big)\ln\Big|\frac{(\omega_{1\sigma}+2T)(\omega_{1\sigma}-2T)}{\omega_{1\sigma}^2}\Big|\\&-i\frac{\pi}{2}|\omega_{1\sigma}|\Big[1-\tanh\Big(\frac{\omega_{1\sigma}}{2T}\Big)\Big]\theta(D+\omega_{1\sigma}).\end{aligned} \tag{S48}$$

Comparing Eqs. (S38), (S43) and (S48), Eqs. (S15)-(S19) can be introduced. In similar way, we can write $I_{4\sigma}^{\alpha(\gamma)}(\omega)=-I_{4\sigma}^{\alpha(\gamma)1}(\omega)+I_{4\sigma}^{\alpha(\gamma)2}(\omega)$ with:

$$I_{4\sigma}^{\alpha(\gamma)1}(\omega)=\int_{-D}^{0}d\varepsilon\frac{\varepsilon\cdot f(\varepsilon-\mu_\alpha)}{\varepsilon+\omega_{2\sigma}+i\delta}, \tag{S49}$$

$$I_{4\sigma}^{\alpha(\gamma)2}(\omega)=\int_0^D d\varepsilon\frac{\varepsilon\cdot f(\varepsilon-\mu_\alpha)}{\varepsilon+\omega_{2\sigma}+i\delta}. \tag{S50}$$

We assume that $0\lesssim\mu_\alpha<D$ and $0\lesssim\omega_{2\sigma}<D'$, one finds:

$$\begin{aligned}I_{4\sigma}^{\alpha(+)1}(\omega)&=\frac{1}{2\beta}\int_{-\beta(D+\mu_\alpha)}^{-\beta\mu_\alpha}\frac{dx(x+\beta\mu_\alpha)}{x+\beta(\mu_\alpha+\omega_{2\sigma})+i\eta}\Big[1-\tanh\Big(\frac{x}{2}\Big)\Big]\\&\approx D-\omega_{2\sigma}\ln\left|\frac{\omega_{2\sigma}}{D-\omega_{2\sigma}}\right|+i\frac{\pi}{2}\omega_{2\sigma}\Big[1+\tanh\Big(\frac{\mu_\alpha+\omega_{2\sigma}}{2T}\Big)\Big]\theta(D-\omega_{2\sigma}),\end{aligned} \tag{S51}$$

$$\begin{aligned}I_{4\sigma}^{\alpha(+)2}(\omega)&\approx\frac{1}{2\beta}\int_{-\beta\mu_\alpha}^{\beta(D-\mu_\alpha)}\frac{dx(x+\beta\mu_\alpha)}{x+\beta(\mu_\alpha+\omega_{2\sigma})}\Big[1-\tanh\Big(\frac{x}{2}\Big)\Big]\approx\mu_\alpha+\omega_{2\sigma}\\&+\omega_{2\sigma}\ln\left|\frac{\omega_{2\sigma}}{\mu_\alpha+\omega_{2\sigma}-2T}\right|+\frac{\omega_{2\sigma}}{2}\Big(1+\frac{\mu_\alpha+\omega_{2\sigma}}{2T}\Big)\ln\left|\frac{\mu_\alpha+\omega_{2\sigma}-2T}{\mu_\alpha+\omega_{2\sigma}+2T}\right|.\end{aligned} \tag{S52}$$

We consider the case $0\lesssim\mu_\alpha<D$ and $-D'<\omega_{2\sigma}\lesssim0$, introducing $\omega_{2\sigma}^+=-\omega_{2\sigma}$, in the same way we have:

$$I_{4\sigma}^{\alpha(+)1}(\omega)\approx\frac{1}{2\beta}\int_{-\beta(D+\mu_\alpha)}^{-\beta\mu_\alpha}\frac{dx(x+\beta\mu_\alpha)}{x+\beta(\mu_\alpha-\omega_{2\sigma}^+)}\Big[1-\tanh\Big(\frac{x}{2}\Big)\Big]\approx D+\omega_{2\sigma}^+\ln\left|\frac{\omega_{2\sigma}^+}{D+\omega_{2\sigma}^+}\right|, \tag{S53}$$

$$\begin{aligned}I_{4\sigma}^{\alpha(+)2}(\omega)&=\frac{1}{2\beta}\int_{-\beta\mu_\alpha}^{\beta(D-\mu_\alpha)}\frac{dx(x+\beta\mu_\alpha)}{x+\beta(\mu_\alpha-\omega_{2\sigma}^+)+i\eta}\Big[1-\tanh\Big(\frac{x}{2}\Big)\Big]\approx\mu_\alpha-\omega_{2\sigma}^++\omega_{2\sigma}^+\ln\left|\frac{\mu_\alpha-\omega_{2\sigma}^+-2T}{\omega_{2\sigma}^+}\right|\\&+\frac{\omega_{2\sigma}^+}{2}\Big(1+\frac{\mu_\alpha-\omega_{2\sigma}^+}{2T}\Big)\ln\left|\frac{\mu_\alpha-\omega_{2\sigma}^++2T}{\mu_\alpha-\omega_{2\sigma}^+-2T}\right|-i\frac{\pi}{2}\omega_{2\sigma}^+\Big[1+\tanh\Big(\frac{\mu_\alpha-\omega_{2\sigma}^+}{2T}\Big)\Big].\end{aligned} \tag{S54}$$

Combining Eqs. (S51)-(S54), we can express the $I_{4\sigma}^{\alpha(+)}$ defined for the entire range of energy, $-D'<\omega_{2\sigma}<D'$:

$$\begin{aligned}I_{4\sigma}^{\alpha(+)}(\omega)&\approx-D+\mu_\alpha+\omega_{2\sigma}+\omega_{2\sigma}\ln\left|\frac{\omega_{2\sigma}^2}{(D-\omega_{2\sigma})(\mu_\alpha+\omega_{2\sigma}-2T)}\right|\\&+\frac{\omega_{2\sigma}}{2}\Big(1+\frac{\mu_\alpha+\omega_{2\sigma}}{2T}\Big)\ln\left|\frac{\mu_\alpha+\omega_{2\sigma}-2T}{\mu_\alpha+\omega_{2\sigma}+2T}\right|-i\frac{\pi}{2}|\omega_{2\sigma}|\Big[1+\tanh\Big(\frac{\mu_\alpha+\omega_{2\sigma}}{2T}\Big)\Big]\theta(D-\omega_{2\sigma}).\end{aligned} \tag{S55}$$

For $-D<\mu_\alpha\lesssim0$ and $0\lesssim\omega_{2\sigma}<D'$ with $\mu_\alpha^+=-\mu_\alpha$ we find:

$$\begin{aligned}I_{4\sigma}^{\alpha(-)1}(\omega)&=\frac{1}{2\beta}\int_{-\beta(D-\mu_\alpha^+)}^{\beta\mu_\alpha^+}\frac{dx(x-\beta\mu_\alpha^+)}{x-\beta(\mu_\alpha^+-\omega_{2\sigma})+i\eta}\Big[1-\tanh\Big(\frac{x}{2}\Big)\Big]\approx D-\mu_\alpha^++\omega_{2\sigma}-\omega_{2\sigma}\ln\left|\frac{\mu_\alpha^+-\omega_{2\sigma}+2T}{D-\omega_{2\sigma}}\right|\\&-\frac{\omega_{2\sigma}}{2}\Big(1-\frac{\mu_\alpha^+-\omega_{2\sigma}}{2T}\Big)\ln\left|\frac{\mu_\alpha^+-\omega_{2\sigma}-2T}{\mu_\alpha^+-\omega_{2\sigma}+2T}\right|+i\frac{\pi}{2}\omega_{2\sigma}\Big[1-\tanh\Big(\frac{\mu_\alpha^+-\omega_{2\sigma}}{2T}\Big)\Big]\theta(D-\omega_{2\sigma}),\end{aligned} \tag{S56}$$

$$I_{4\sigma}^{\alpha(-)2}(\omega)\approx\frac{1}{2\beta}\int_{\beta\mu_\alpha^+}^{\beta(D+\mu_\alpha^+)}\frac{dx(x-\beta\mu_\alpha^+)}{x-\beta(\mu_\alpha^+-\omega_{2\sigma})}\Big[1-\tanh\Big(\frac{x}{2}\Big)\Big]\approx0. \tag{S57}$$

In the case of $-D<\mu_\alpha\lesssim0$ and $-D'<\omega_{2\sigma}\lesssim0$ we have:

$$\begin{aligned}I_{4\sigma}^{\alpha(-)1}(\omega)&\approx\frac{1}{2\beta}\int_{-\beta(D-\mu_\alpha^+)}^{\beta\mu_\alpha^+}\frac{dx(x-\beta\mu_\alpha^+)}{x-\beta(\mu_\alpha^++\omega_{2\sigma}^+)}\Big[1-\tanh\Big(\frac{x}{2}\Big)\Big]\approx D-\mu_\alpha^+-\omega_{2\sigma}^+\\&+\omega_{2\sigma}^+\ln\left|\frac{\mu_\alpha^++\omega_{2\sigma}^++2T}{D+\omega_{2\sigma}^+}\right|+\frac{\omega_{2\sigma}^+}{2}\Big(1-\frac{\mu_\alpha^++\omega_{2\sigma}^+}{2T}\Big)\ln\left|\frac{\mu_\alpha^++\omega_{2\sigma}^+-2T}{\mu_\alpha^++\omega_{2\sigma}^++2T}\right|,\end{aligned} \tag{S58}$$

$$I_{4\sigma}^{\alpha(-)2}(\omega)=\frac{1}{2\beta}\int_{\beta\mu_\alpha^+}^{\beta(D+\mu_\alpha^+)}\frac{dx(x-\beta\mu_\alpha^+)}{x-\beta(\mu_\alpha^++\omega_{2\sigma}^+)+i\eta}\Big[1-\tan\Big(\frac{x}{2}\Big)\Big]\approx-i\frac{\pi}{2}\omega_{2\sigma}^+\Big[1-\tanh\Big(\frac{\mu_\alpha^++\omega_{2\sigma}^+}{2T}\Big)\Big]. \tag{S59}$$

Using Eqs. (S56)-(S59), we obtain $I_{4\sigma}^{\alpha(-)}$ for $-D' < \omega_{2\sigma} < D'$:

$$I_{4\sigma}^{\alpha(-)}(\omega) \approx -D - \mu_\alpha - \omega_{2\sigma} + \omega_{2\sigma}\ln\left|\frac{\mu_\alpha + \omega_{2\sigma} - 2T}{D - \omega_{2\sigma}}\right| + \frac{\omega_{2\sigma}}{2}\left(1 + \frac{\mu_\alpha + \omega_{2\sigma}}{2T}\right)\ln\left|\frac{\mu_\alpha + \omega_{2\sigma} + 2T}{\mu_\alpha + \omega_{2\sigma} - 2T}\right| \\ - i\frac{\pi}{2}|\omega_{2\sigma}|\Big[1 + \tanh\left(\frac{\mu_\alpha + \omega_{2\sigma}}{2T}\right)\Big]\theta(D - \omega_{2\sigma}). \tag{S60}$$

We now take the case $\mu_\alpha = 0$ and $0 \lesssim \omega_{2\sigma} < D'$ and find:

$$I_{4\sigma}^{\alpha(0)1}(\omega) = \frac{1}{2\beta}\int_{-\beta D}^{0}\frac{xdx}{x + \beta\omega_{2\sigma} + i\eta}\Big[1 - \tanh\left(\frac{x}{2}\right)\Big] \approx D - \frac{T}{2} + \frac{\omega_{2\sigma}}{2} - \omega_{2\sigma}\ln\left|\frac{\omega_{2\sigma} - 2T}{D - \omega_{2\sigma}}\right| \\ - \frac{\omega_{2\sigma}}{2}\left(1 + \frac{\omega_{2\sigma}}{2T}\right)\ln\left|\frac{\omega_{2\sigma}}{\omega_{2\sigma} - 2T}\right| + i\frac{\pi}{2}\omega_{2\sigma}\Big[1 + \tanh\left(\frac{\omega_{2\sigma}}{2T}\right)\Big]\theta(D - \omega_{2\sigma}), \tag{S61}$$

$$I_{4\sigma}^{\alpha(0)2}(\omega) \approx \frac{1}{2\beta}\int_{0}^{\beta D}\frac{xdx}{x + \beta\omega_{2\sigma}}\Big[1 - \tanh\left(\frac{x}{2}\right)\Big] \approx \frac{T}{2} + \frac{\omega_{2\sigma}}{2} - \frac{\omega_{2\sigma}}{2}\left(1 + \frac{\omega_{2\sigma}}{2T}\right)\ln\left|\frac{\omega_{2\sigma} + 2T}{\omega_{2\sigma}}\right|. \tag{S62}$$

For $\mu_\alpha = 0$ and $-D' < \omega_{2\sigma} \lesssim 0$ with $\omega_{2\sigma}^{+} = -\omega_{2\sigma}$, we obtain:

$$I_{4\sigma}^{\alpha(0)1}(\omega) \approx \frac{1}{2\beta}\int_{-\beta D}^{0}\frac{xdx}{x - \beta\omega_{2\sigma}^{+}}\Big[1 - \tanh\left(\frac{x}{2}\right)\Big] \approx D - \frac{T}{2} - \frac{\omega_{2\sigma}^{+}}{2} \\ + \frac{\omega_{2\sigma}^{+}}{2}\left(1 - \frac{\omega_{2\sigma}^{+}}{2T}\right)\ln\left|\frac{\omega_{2\sigma}^{+}}{\omega_{2\sigma}^{+} + 2T}\right| + \omega_{2\sigma}^{+}\ln\left|\frac{\omega_{2\sigma}^{+} + 2T}{D + \omega_{2\sigma}^{+}}\right|, \tag{S63}$$

$$I_{4\sigma}^{\alpha(0)2}(\omega) = \frac{1}{2\beta}\int_{0}^{\beta D}\frac{xdx}{x - \beta\omega_{2\sigma}^{+} + i\eta}\Big[1 - \tanh\left(\frac{x}{2}\right)\Big] \approx \frac{T}{2} - \frac{\omega_{2\sigma}^{+}}{2} \\ + \frac{\omega_{2\sigma}^{+}}{2}\left(1 - \frac{\omega_{2\sigma}^{+}}{2T}\right)\ln\left|\frac{\omega_{2\sigma}^{+} - 2T}{\omega_{2\sigma}^{+}}\right| - i\frac{\pi}{2}\omega_{2\sigma}^{+}\Big[1 - \tanh\left(\frac{\omega_{2\sigma}^{+}}{2T}\right)\Big]. \tag{S64}$$

Comparing Eqs. (S61)-(S62) with Eqs. (S63)-(S64), one finds the $I_{4\sigma}^{\alpha(0)}$ for the full energy domain:

$$I_{4\sigma}^{\alpha(0)}(\omega) \approx -D + T + \omega_{2\sigma}\ln\left|\frac{\omega_{2\sigma} - 2T}{D - \omega_{2\sigma}}\right| + \frac{\omega_{2\sigma}}{2}\left(1 + \frac{\omega_{2\sigma}}{2T}\right)\ln\left|\frac{\omega_{2\sigma}^2}{(\omega_{2\sigma} - 2T)(\omega_{2\sigma} + 2T)}\right| \\ - i\frac{\pi}{2}|\omega_{2\sigma}|\Big[1 + \tanh\left(\frac{\omega_{2\sigma}}{2T}\right)\Big]\theta(D - \omega_{2\sigma}). \tag{S65}$$

In the same way, comparing Eqs. (S55), (S60) and (S65), Eqs. (S20)-(S24) can be introduced.

Note that these results are valid as well at low temperatures. For absolute zero temperature we can substitute $f_\alpha(\varepsilon_k)$ with the Heaviside function, i.e., $f_\alpha(\varepsilon_k) = \theta(\mu_\alpha - \varepsilon_k)$, and using the method presented above the integrals can be calculated.

### Appendix C: The verification of an analytical solution

In this section, we compare our analytical results for $\Sigma_{3\sigma}(\omega)$ presented in Appendix B with those of Z.-G. Zhu and J. Berakdar in Ref. [7]. In order to do this, we introduce the following integral:

$$I(\omega) = \int_{-D}^{D} d\varepsilon \frac{|\varepsilon| f(\varepsilon - \mu)}{-\varepsilon + \omega + i\delta}. \tag{S66}$$

Z.-G. Zhu and J. Berakdar applied a contour integral method in complex plane and found that:

$$I(\omega) = \frac{|D|}{2}\ln\left(\frac{|D^2 - \omega^2|}{(2\pi T)^2}\right) - |\mu|\psi(z) - \frac{1}{2}\Big[\omega\ln\frac{|D^2 - \omega^2|}{\omega^2} + i\pi|\omega|\theta(D - |\omega|)\Big], \tag{S67}$$

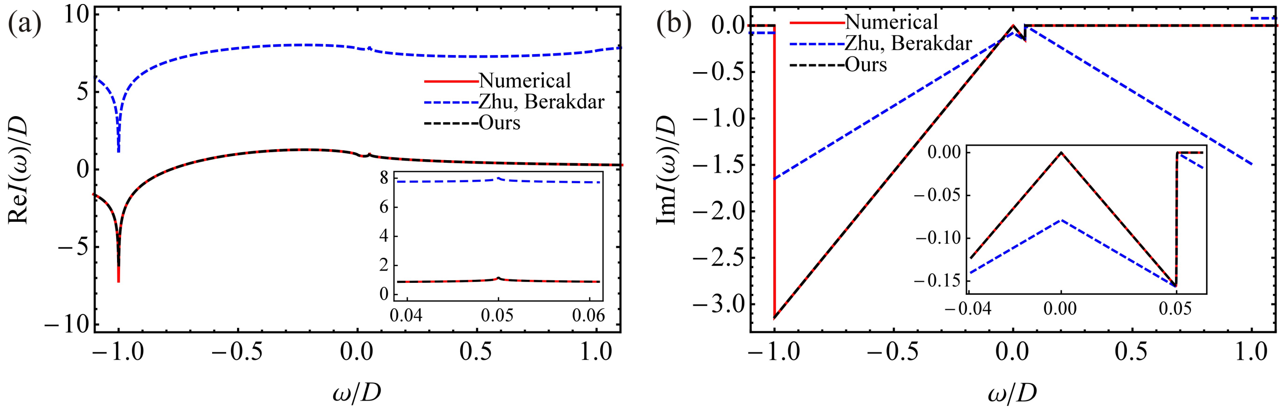


FIG. S1. (a) Real part of $I(\omega)$ as a function of energy. (b) Imaginary part of $I(\omega)$ as a function of energy. The chemical potential is fixed at $\mu/D = 0.05$ and the temperature is set to be $T/D = 5 \cdot 10^{-5}$. It can be observed that our analytical results show a good agreement with the numerical calculations. The results of Z.-G. Zhu and J. Berakdar present a departure from the numerical calculations due to the mathematical method used by them.

where $z = \frac{1}{2} + \frac{\omega - \mu}{2\pi i T}$ and $\psi(z)$ is the digamma function. It can be shown that the integrating function in Eq. (S66) is not a holomorphic function, and thus the contour integral method can not be applied for $I(\omega)$. As we shall see, their results differ from those obtained by numerical calculations (see Figure S1). Our analytical results, given by $I_{3\sigma}^{\alpha(+)}(\omega)$ in Appendix B, are in better agreement with the numerical calculations. Therefore, it can be verified that the relation (S67) does not accurately reproduce the case of the absolute zero temperature.

[1] J. S. Lim, R. López, L. Limot, and P. Simon, Phys. Rev. B **88**, 165403 (2013).
[2] C. Lacroix, J. Phys. F: Met. Phys. **11**, 2389 (1981).
[3] V. Kashcheyevs, A. Aharony, and O. Entin-Wohlman, Phys. Rev. B **73**, 125338 (2006).
[4] Y. Meir, N. S. Wingreen, and P. A. Lee, Phys. Rev. Lett. **66**, 3048 (1991).
[5] I. S. Gradshteyn and I. M. Ryzhik, *Table of integrals, series, and products*, seventh ed. (Academic Press: Cambridge, Massachusetts, USA, 2007) p. 42.
[6] W. Nolting, *Fundamentals of Many-body Physics: Principles and Methods* (Springer-Verlag: Berlin, Germany, 2009) p. 140.
[7] Z.-G. Zhu and J. Berakdar, Phys. Rev. B **84**, 165105 (2011).
